# Supplementary material for: Analysis of NaN Divergence in Training Monocular Depth Estimation Model
Source: arXiv:2311.03938 source file (2023-11-07)
Supplement: Supplementary file 1 [file X_suppl.tex]

%\clearpage
\setcounter{page}{1}
\maketitlesupplementary

\section{More Details on $\epsilon$}
In the main text, we mentioned that $\epsilon \leq 7.0 \times 10^{-46}$ yielded a NaN loss because it was smaller than the representable float. Here, we detail this behavior.

We consider FP32 of PyTorch. Here, $\epsilon$ is added only in the training phase for computing the scale-invariant log loss. Using the built-in function \texttt{torch.finfo()}, which describes information on precision type, we obtain

\ \\
\texttt{>>> torch.finfo(torch.float32)} \\
\texttt{finfo(resolution=1e-06, min=-3.40282e+38, max=3.40282e+38, eps=1.19209e-07, tiny=1.17549e-38, dtype=float32)}
\ \\

In practice, the product of \texttt{eps} and $\texttt{tiny}$, which is about $1.4013 \times 10^{-45}$, becomes the smallest representable float in PyTorch. Note that the value is different from the smallest representable float in Python. For example,

\ \\
\texttt{>>> torch.Tensor([7.1e-46])} \\
\texttt{tensor([1.4013e-45])} \\
\texttt{>>> torch.Tensor([7.0e-46])} \\
\texttt{tensor([0.])}
\ \\

This behavior means that $1.4013 \times 10^{-45}$ becomes the smallest boundary when casting Python float into PyTorch float. When using Python float $\epsilon \leq 7.0 \times 10^{-46}$, it is converted to zero in PyTorch float, which results in a NaN in the logarithmic function.

From this behavior, we know that using an extremely smaller value such as $\epsilon=10^{-40}$ for the logarithmic function may work. However, we recommend having enough margin from the smallest float by using $\epsilon=10^{-24}$ because this value provides sufficient properties, such as gradient scale.

On various GPU machines and PyTorch versions, we obtained consistent results from the above test.

\section{Dataset Statistics}
Note that the gradient is affected by the ground-truth depth map, and therefore, using different ground-truths changes the gradient. To perform realistic simulations, we generated artificial data following the mean and standard deviation of \{KITTI, NYU-Depth V2, Driving Stereo, Argoverse, DDAD\}. \tabref{tab:meanstd} summarizes the mean and standard deviation of the ground-truth depth for the five datasets. Additionally, we removed negative depths that were accidentally generated, while we observed that ignoring them hardly influenced the mean and standard deviation of the generated samples.

\begin{table}[t!]
	\centering
	\begin{tabular}{l|rr}
		\toprule
		\textbf{Dataset} & \multicolumn{1}{l}{\textbf{Mean}} & \multicolumn{1}{l}{\textbf{Std}} \\
		\midrule
		KITTI            & 16.2307                           & 5.3810                           \\
		NYU-Depth V2     & 2.8497                            & 1.2845                           \\
		Driving Stereo   & 23.8313                           & 7.7740                           \\
		Argoverse        & 26.1697                           & 1.9219                           \\
		DDAD             & 31.4102                           & 3.2712                           \\
		\bottomrule
	\end{tabular}
	\caption{We measured the mean and standard deviation of the ground-truth depth for the five datasets. All values are in meters.}
	\label{tab:meanstd}
\end{table}
